# Supplementary material for: Voltage-dependent cluster expansion for electrified solid-liquid interfaces: Application to the electrochemical deposition of transition metals
Source: arXiv:1708.03407 ancillary file (2017-11-07)
Supplement: Supplementary file 1 [file Supplemental_Information.pdf]

# Supplemental information for "Voltage-dependent cluster expansion for electrified solid-liquid interfaces: Application to the electrochemical deposition of transition metals"

Stephen E. Weitzner* and Ismaila Dabo

*Department of Materials Science and Engineering,*

*Materials Research Institute,*

*and Penn State Institutes of Energy and the Environment,*

*The Pennsylvania State University,*

*University Park, PA 16802, USA*

*Email: weitzner@psu.edu*

## S1. CONFIGURATIONAL DATA

Here we provide details of the dataset used to parameterize the cluster expansion presented in this work. The surface coverage $\theta$, the neutral surface binding energy $F_0(\boldsymbol{\sigma})$ (referred to bulk silver), the potential of zero charge $\Phi_0$, the *ab initio* capacitance of the interface $C_0$, and the surface area $A$ for each configuration $\boldsymbol{\sigma}$ are summarized below in Table S1.1. Details regarding the calculation of the differential capacitance are provided in the following section.

TABLE S1.1: Thermodynamic data of the configurations considered in the Letter. Capacitance values are reported for a Helmholtz width of 3 Å referred to the silver layer. Silver adatoms are shown in blue and the surface unit cell is shown in red.

| $\boldsymbol{\sigma}$ | $\theta$ | $F_0(\boldsymbol{\sigma})$ [meV/site] | $\Phi_0$ [V] | $\Phi_0$ [V/SHE] | $C_0$ [$\mu$F/cm$^2$] | A [Å$^2$] |
|---|---|---|---|---|---|---|
| 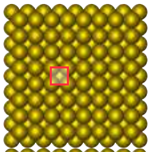 | 0 | 0 | 4.95 | 0.24 | 13.56 | 8.70 |
| 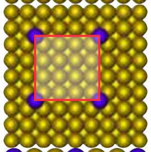 | 0.0625 | −1.78 | 4.69 | −0.02 | 14.13 | 139.21 |
| 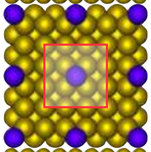 | 0.11 | 0.51 | 4.53 | −0.18 | 15.01 | 78.31 |
| 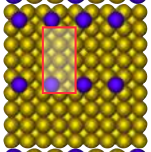 | 0.125 | 2.64 | 4.47 | −0.24 | 15.44 | 69.61 |
| 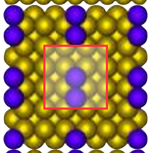 | 0.22 | −1.58 | 4.35 | −0.36 | 16.57 | 78.31 |
| 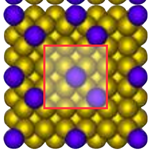 | 0.22 | 13.55 | 4.23 | −0.48 | 16.89 | 78.31 |

Continued . . .

TABLE S1.1: Continued

| $\boldsymbol{\sigma}$ | $\theta$ | $F_0(\boldsymbol{\sigma})$ [meV/site] | $\Phi_0$ [V] | $\Phi_0$ [V vs. SHE] | $C_0$ [$\mu$F/cm$^2$] | A [Å$^2$] |
|---|---|---|---|---|---|---|
| 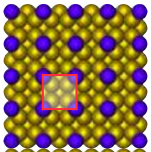 | 0.25 | 16.46 | 4.17 | −0.54 | 17.08 | 34.81 |
| 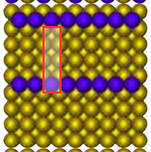 | 0.25 | −16.02 | 4.48 | −0.23 | 18.67 | 34.81 |
| 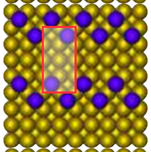 | 0.25 | 19.17 | 4.18 | −0.53 | 17.52 | 69.61 |
| 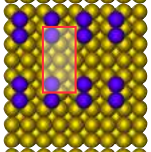 | 0.25 | 2.75 | 4.30 | −0.40 | 18.73 | 69.61 |
| 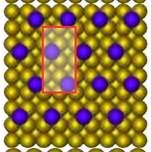 | 0.25 | 17.54 | 4.15 | −0.56 | 16.94 | 69.61 |
| 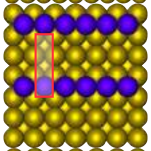 | 0.33 | −17.40 | 4.31 | −0.40 | 17.91 | 26.10 |
| 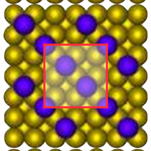 | 0.33 | 33.40 | 4.00 | −0.71 | 18.78 | 78.31 |
| 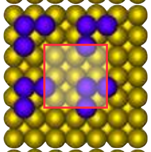 | 0.33 | 3.17 | 4.18 | −0.53 | 18.35 | 78.31 |
| 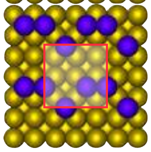 | 0.33 | 15.79 | 4.10 | −0.60 | 18.59 | 78.31 |

Continued . . .

TABLE S1.1: Continued

| $\boldsymbol{\sigma}$ | $\theta$ | $F_0(\boldsymbol{\sigma})$ [meV/site] | $\Phi_0$ [V] | $\Phi_0$ [V vs. SHE] | $C_0$ [$\mu$F/cm$^2$] | A [Å$^2$] |
|---|---|---|---|---|---|---|
| 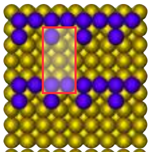 | 0.375 | −12.17 | 4.24 | −0.47 | 17.80 | 69.61 |
| 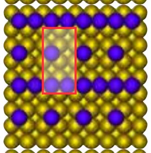 | 0.375 | 1.02 | 4.11 | −0.60 | 18.05 | 69.61 |
| 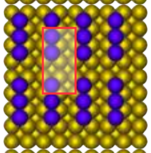 | 0.375 | 3.44 | 4.12 | −0.59 | 18.45 | 69.61 |
| 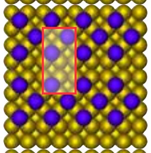 | 0.375 | 40.71 | 3.90 | −0.81 | 18.82 | 69.61 |
| 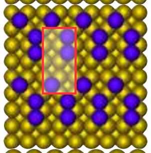 | 0.375 | 23.54 | 4.01 | −0.70 | 19.00 | 69.61 |
| 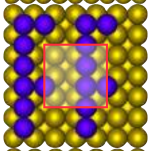 | 0.44 | −10.19 | 4.15 | −0.56 | 19.17 | 78.31 |
| 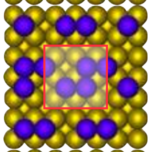 | 0.44 | −1.34 | 4.07 | −0.58 | 19.47 | 76.31 |
| 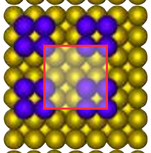 | 0.44 | 7.62 | 4.13 | −0.64 | 19.19 | 78.31 |
| 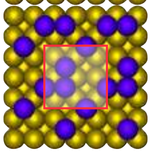 | 0.44 | 21.71 | 3.98 | −0.72 | 19.31 | 78.31 |

Continued . . .

TABLE S1.1: Continued

| $\boldsymbol{\sigma}$ | $\theta$ | $F_0(\boldsymbol{\sigma})$ [meV/site] | $\Phi_0$ [V] | $\Phi_0$ [V vs. SHE] | $C_0$ [$\mu$F/cm$^2$] | A [Å$^2$] |
|---|---|---|---|---|---|---|
| 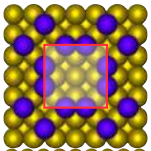 | 0.44 | 17.91 | 4.00 | −0.71 | 19.46 | 78.31 |
| 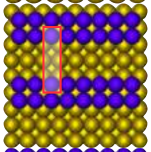 | 0.50 | −35.14 | 4.27 | −0.44 | 18.43 | 34.81 |
| 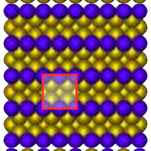 | 0.50 | −8.00 | 4.06 | −0.64 | 20.15 | 34.81 |
| 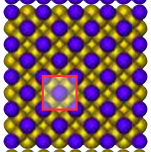 | 0.50 | 69.35 | 3.69 | −1.02 | 19.82 | 34.81 |
| 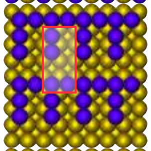 | 0.50 | −6.56 | 4.06 | −0.64 | 19.59 | 69.61 |
| 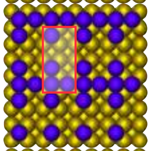 | 0.50 | −5.14 | 4.04 | −0.67 | 18.90 | 69.61 |
| 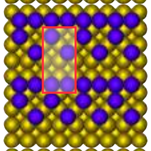 | 0.50 | 11.64 | 3.96 | −0.75 | 19.49 | 69.61 |
| 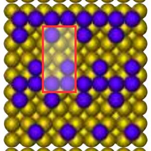 | 0.50 | −4.32 | 4.05 | −0.66 | 19.03 | 69.61 |
| 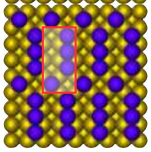 | 0.50 | 29.62 | 3.89 | −0.81 | 20.35 | 69.61 |

Continued ...

TABLE S1.1: Continued

| $\boldsymbol{\sigma}$ | $\theta$ | $F_0(\boldsymbol{\sigma})$ [meV/site] | $\Phi_0$ [V] | $\Phi_0$ [V vs. SHE] | $C_0$ [$\mu$F/cm$^2$] | A [Å$^2$] |
|---|---|---|---|---|---|---|
| 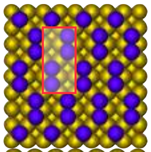 | 0.50 | 31.10 | 3.92 | −0.79 | 20.75 | 69.61 |
| 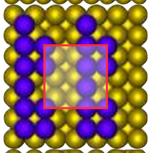 | 0.55 | −14.13 | 4.09 | −0.62 | 19.39 | 78.31 |
| 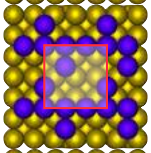 | 0.55 | −3.36 | 4.01 | −0.70 | 19.27 | 78.31 |
| 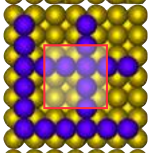 | 0.55 | −21.48 | 4.10 | −0.60 | 19.86 | 78.31 |
| 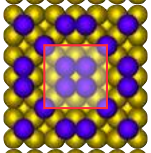 | 0.55 | 16.04 | 3.92 | −0.79 | 19.28 | 78.31 |
| 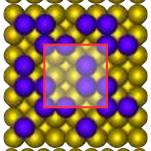 | 0.55 | 12.27 | 3.94 | −0.77 | 19.62 | 78.31 |
| 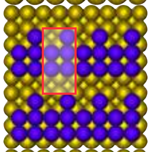 | 0.625 | −28.63 | 4.07 | −0.64 | 18.77 | 69.61 |
| 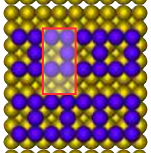 | 0.625 | −14.94 | 4.02 | −0.69 | 20.35 | 69.61 |
| 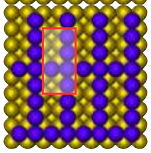 | 0.625 | −15.06 | 4.02 | −0.69 | 20.62 | 69.61 |

Continued . . .

TABLE S1.1: Continued

| $\boldsymbol{\sigma}$ | $\theta$ | $F_0(\boldsymbol{\sigma})$ [meV/site] | $\Phi_0$ [V] | $\Phi_0$ [V vs. SHE] | $C_0$ [$\mu$F/cm$^2$] | A [Å$^2$] |
|---|---|---|---|---|---|---|
| 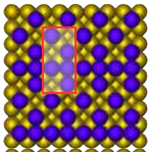 | 0.625 | 21.66 | 3.82 | −0.89 | 19.78 | 69.61 |
| 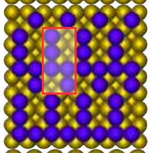 | 0.625 | 2.28 | 3.94 | −0.77 | 20.31 | 69.61 |
| 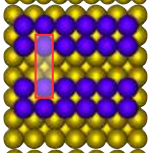 | 0.66 | −33.36 | 4.09 | −0.62 | 19.11 | 26.10 |
| 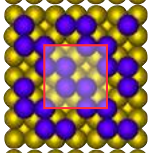 | 0.66 | 4.84 | 3.89 | −0.81 | 20.03 | 78.31 |
| 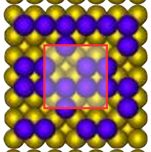 | 0.66 | −8.18 | 3.94 | −0.76 | 19.67 | 78.31 |
| 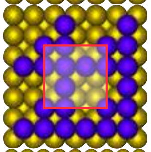 | 0.66 | −24.61 | 4.03 | −0.68 | 19.71 | 78.31 |
| 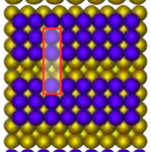 | 0.75 | −50.73 | 4.07 | −0.64 | 19.22 | 34.80 |
| 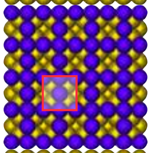 | 0.75 | −23.28 | 3.96 | −0.75 | 20.48 | 34.80 |
| 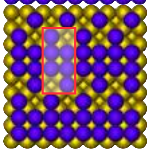 | 0.75 | −20.67 | 3.92 | −0.79 | 19.60 | 69.61 |

Continued . . .

TABLE S1.1: Continued

| $\boldsymbol{\sigma}$ | $\theta$ | $F_0(\boldsymbol{\sigma})$ [meV/site] | $\Phi_0$ [V] | $\Phi_0$ [V vs. SHE] | $C_0$ [$\mu$F/cm$^2$] | A [Å$^2$] |
|---|---|---|---|---|---|---|
| 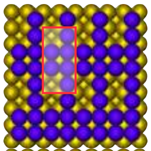 | 0.75 | −38.11 | 4.02 | −0.69 | 20.09 | 69.61 |
| 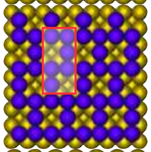 | 0.75 | −24.99 | 3.98 | −0.73 | 20.45 | 69.61 |
| 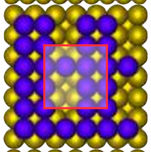 | 0.77 | −43.71 | 4.02 | −0.68 | 19.61 | 78.31 |
| 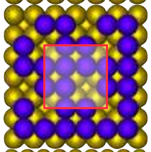 | 0.77 | −29.57 | 3.96 | −0.75 | 19.74 | 78.31 |
| 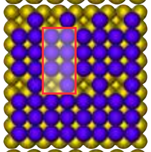 | 0.875 | −62.03 | 4.03 | −0.68 | 19.47 | 69.61 |
| 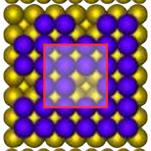 | 0.88 | −64.87 | 4.03 | −0.68 | 19.29 | 78.31 |
| 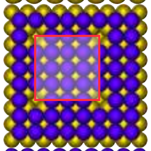 | 0.9375 | −81.82 | 4.05 | −0.65 | 18.84 | 139.21 |
| 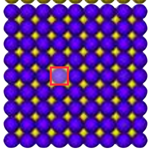 | 1.00 | −101.29 | 4.08 | −0.63 | 18.34 | 8.70 |

## S2. DIFFERENTIAL CAPACITANCE FROM FIRST PRINCIPLES

The capacitance of each surface cell is computed at the level of the quantum-continuum model by adding explicit charges along the surface and incorporating a planar Gaussian ionic countercharge several angstroms from the surface within the continuum solvent. We note that the Gaussian plane model is appropriate for representing systems in the limit of concentrated electrolytes, where, for the example of a monovalent electrolyte, the Debye length of the electrical double layer approaches $3-5$ Å from the electrode surface for concentrations between $1-0.35$ M. The equilibrium voltage on the charged slabs are then extracted as the opposite of the Fermi level after aligning the converged potentials to zero at the edge of the supercell. To illustrate this, we show the effects of the surface charge on the electrostatic potential of the $c(2\times 2)$ configuration from Table S1.1 below in Fig. S2.1. Calculating the

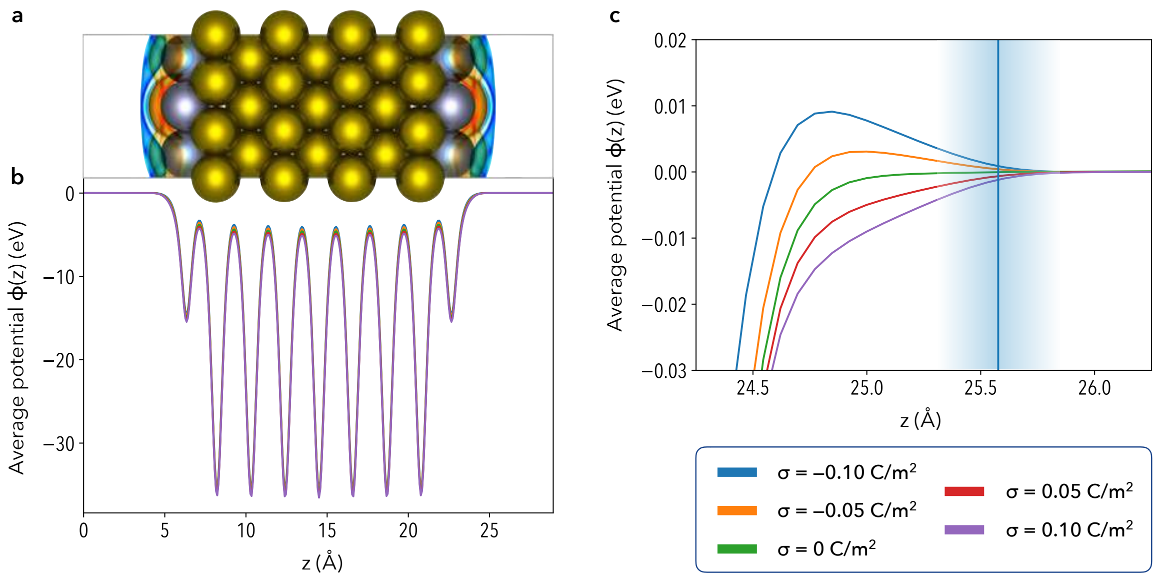


FIG. S2.1. The finite charges placed on the solvated $c(2\times 2)$ slab are screened by the planar ionic countercharge in solution. (a) The response of the continuum dielectric at the cavity interface is visualized. Positive/negative polarization charges are shown in red/blue. (b) The electrostatic potentials of the electrified slabs are aligned to zero at the edges of the supercell. (c) The planar (Gaussian) ionic countercharge positioned 3 Å from the silver adlayer screens the surface charge $\sigma$, providing a suitable reference level in the bulk of the solvent to extract charge-dependent voltages.

derivative of Eq. 6 from the Letter with respect to the charge in the system, we derive the charge-dependent voltage

$$\Phi(\boldsymbol{\sigma}, Q) = \Phi_0 + \frac{Q}{AC_0}. \tag{S2.1}$$

Using Eq. S2.1, we obtain the differential capacitance of each interface via linear regression for a fixed countercharge position. In Fig. S2.2, we show the effect of varying the thickness of the double layer when it is referred to either the position of the silver adlayer or the topmost gold layer. Decreasing the double layer thickness leads to a proportional increase in the

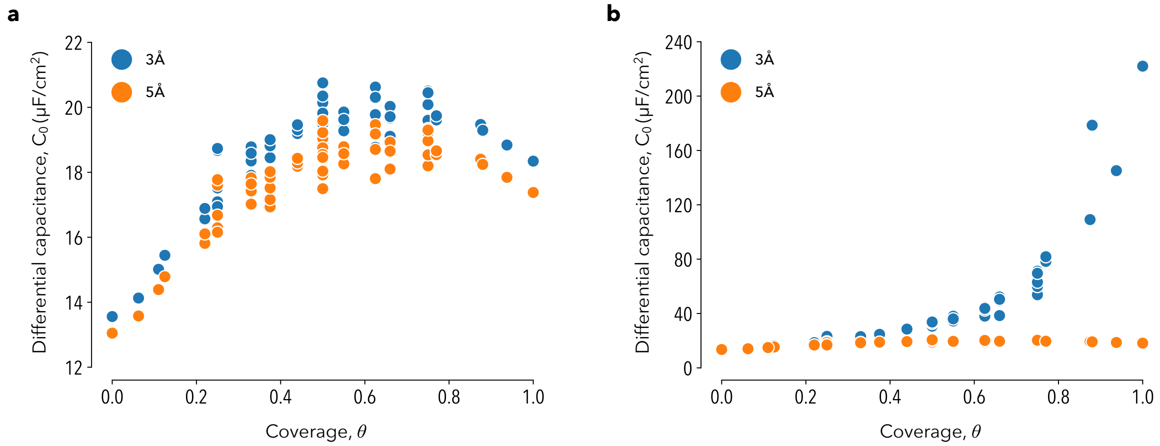


FIG. S2.2. Differential capacitance data for the configurations presented in Table S1.1 referred to (a) the silver adlayer position and (b) the topmost gold layer.

capacitance as anticipated from the linear definition of the ionic countercharge. In the case of the gold layer reference, we find that positioning the planar countercharge at 3 Å places the charge within the silver adlayer, leading to artificially large values of the capacitance. This effect is especially apparent at higher coverages, as shown in Fig. S2.2b.

## S3. CLUSTER EXPANSION FITTING

Cluster expansions were constructed by considering clusters with diameters up to fourth nearest neighbors and that sample up to four sites. Each cluster was added to the expansion only after all clusters of a smaller diameter were present and all of the sub-clusters were already included in the expansion, as shown in Fig. S3.3. The leave one out cross validation

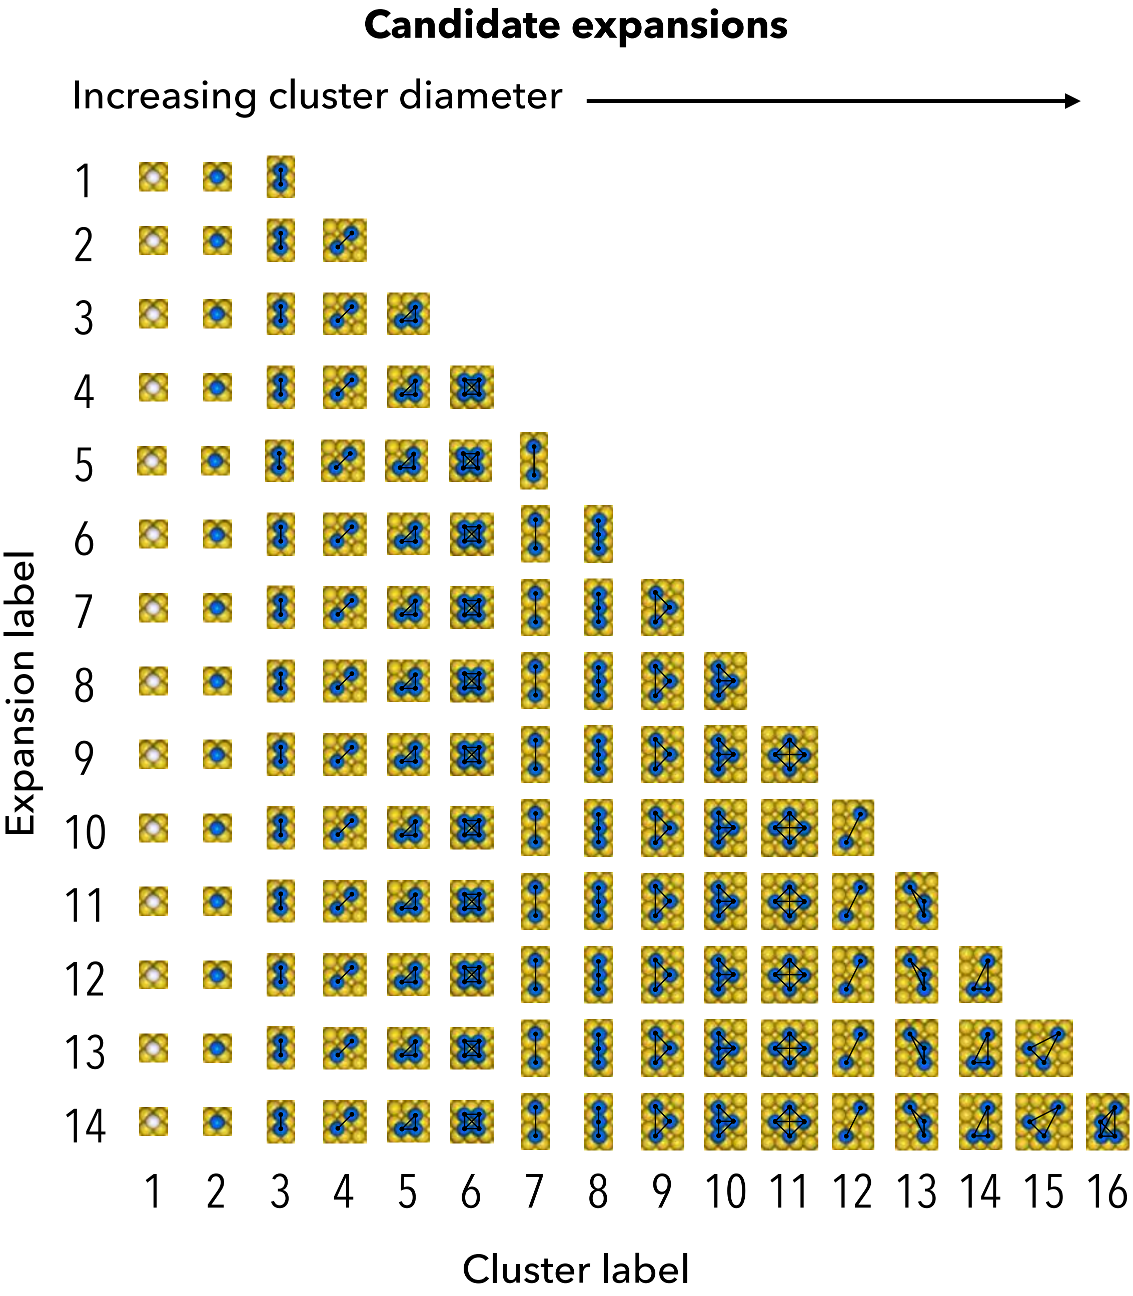


FIG. S3.3. Candidate expansions considered in this work.

(LOOCV) score

$$\Delta = \left( k^{-1} \sum_{i}^{k} (\mathscr{F}_i - \hat{\mathscr{F}}_i)^2 \right)^{\frac{1}{2}} \tag{S3.2}$$

was computed with each expansion for different values of the interfacial capacitance. Below in Fig S3.4 we show the convergence in the LOOCV score for capacitance values of 0 $\mu$F/cm$^2$

and 30 $\mu$F/cm$^2$. Here we observe that the accuracy of the expansions are well converged by

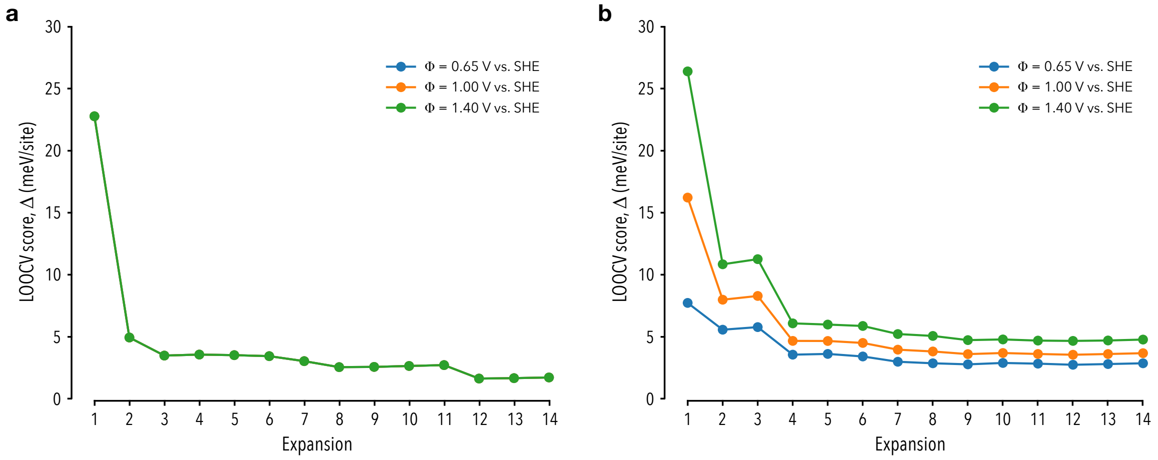


FIG. S3.4. Leave one out cross validation scores computed for candidate expansion at voltages of 0.65 V, 1.00 V, and 1.40 V vs. SHE for capacitance values of (a) 0 $\mu$F/cm$^2$ and (b) 30 $\mu$F/cm$^2$.

expansion 12 (*c.f.*, Fig S3.3); however, we made the conservative choice to select expansion 14 for this work due to the sensitivity of the accuracy to the applied voltage as shown in panel b in Fig. S3.4.

In Fig. S3.5, we show the computed effective cluster interaction values for expansion 14 at a capacitance value of 30 $\mu$F/cm$^2$. We find that point clusters contribute strongly within the entire considered voltage range and that their contribution increases with increasing voltage. Furthermore, clusters with a diameter less than two nearest neighbors appear to be the most important for describing the energy of different adlayer configurations, while larger clusters contribute to a lesser extent. The latter is also evident when studying the LOOCV scores in Fig. S3.4, as the accuracy of the expansions increase rapidly as small clusters with diameters up to two nearest neighbors are introduced, but then gradually converges with the addition of larger clusters.

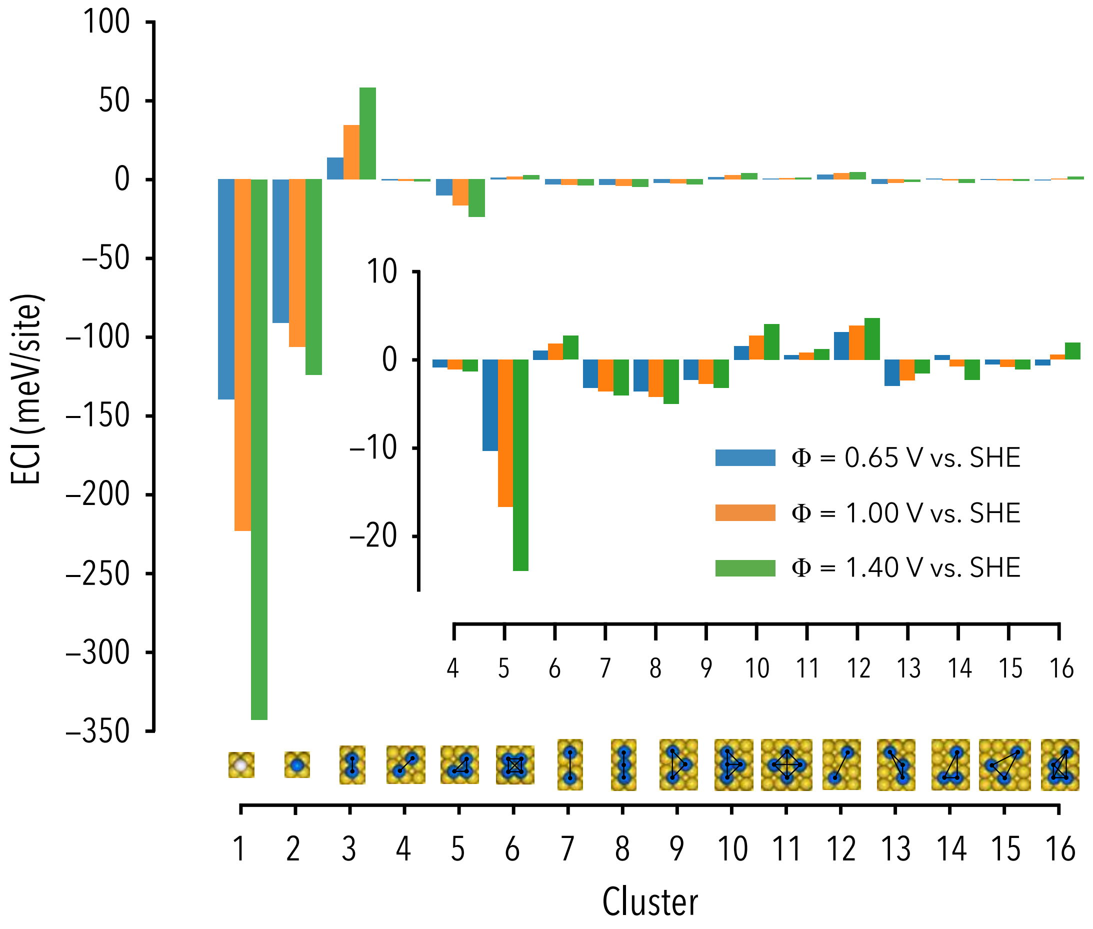


FIG. S3.5. Effective cluster interactions (ECI) obtained for expansion 14 via linear regression across the entire dataset in Table S1.1 for a capacitance value of 30 $\mu$F/cm$^2$. For each cluster, we show the ECI values obtained at voltages of 0.65 V, 1.00 V, and 1.40 V vs. SHE from left to right (blue, orange, green), respectively. In the inset, we show the effects of the applied voltage on the ECI values of the larger clusters.
